# Supplementary material for: First-order Conditions for Optimization in the Wasserstein Space
Source: arXiv:2209.12197 source file (2025-02-28)
Supplement: Supplementary file 1 [file supplement_dro.tex]

\section{Relation to Existing Results in \gls{acr:dro}}
Consider the cost function
\begin{equation*}
    \cost(w,\mu)=\expectedValue{\mu}{f(w,x)},
\end{equation*}
and suppose that, for fixed $w$, $f$ is twice continuously differentiable in $x$ and has at most quadratic growth\footnote{Again, one can relax this assumption by requiring that the positive part of $f$ has at most quadratic growth; see discussion in \cref{prop:expectation}}. To ease the notation we will simply write $f(x)$, omitting the dependency on $w$.
We define the \emph{growth rate} of $f$~\cite{Gao2016} as
\begin{equation*}
    \kappa\coloneqq\limsup_{\norm{x}\to\infty}\frac{f(x)}{\norm{x}^2}.
\end{equation*}
Without loss of generality, we assume that $\kappa<+\infty$ or, equivalently, that the supremum is finite; see \cite[Theorem 2]{Yue2021}, \cite[Theorem 1 and Proposition 2]{Gao2016}, and~\cite[Remark 3]{Blanchet2019}. 
Note that, if $f$ has at most quadratic growth, then $\kappa<+\infty$.
Then, by duality for \gls{acr:dro} (see \cite[Theorem 1]{Blanchet2019} and \cite[Theorem 1]{Gao2016}), we have
\begin{equation}\label{eq:dro reformulation}
    \sup_{\mu\in\closedWassersteinBall{2}{\radius}{\refmu}}\expectedValue{\mu}{f(x)}
    =
    \min_{\lambda\geq 0}\lambda\radius^2-\int_{\reals^d}\inf_{x'\in\reals^d}\lambda\Vert x-x'\Vert^2-f(x')\d\refmu(x).
\end{equation}
We assume the supremum is attained by some distribution $\mu^\ast$, and that the solution of the unconstrained problem (i.e., without the constraint $\mu\in\closedWassersteinBall{2}{\radius}{\refmu}$) is not feasible. In turn, this assumptions implies that alla maxima lie at the boundary of the Wasserstein ball and that $\lambda^\ast>0$; see~\cite[Remark 2]{Blanchet2019}.
Moreover, we assume that the growth rate $\kappa$ provides a uniform upper bound for the largest eigenvalue of the Hessian of $f$:
\begin{equation*}
    \kappa\geq\sup_{x\in\reals^d}\frac{\maxEigenvalue{\gradient{}^2f(x)}}{2}.
\end{equation*}
By the following lemma, we can in fact replace the inequality with an equality:
\begin{lemma}
Let $f\in\Ctwo{\reals^d}$ have growth rate $\kappa<+\infty$. 
Assume $\kappa\geq\sup_{x\in\reals^d}\frac{\maxEigenvalue{\gradient{}^2f(x)}}{2}$. Then, 
\begin{equation*}
    \kappa=\sup_{x\in\reals^d}\frac{\maxEigenvalue{\gradient{}^2f(x)}}{2}.
\end{equation*}
\end{lemma}
\begin{proof}
It suffices to prove one inequality. By (multivariate) Taylor's remainder formula
\begin{equation*}
    f(x)=f(0)+\innerProduct{\gradient{}f(0)}{x} + R(x)
    \quad
    \text{with}
    \quad 
    R(x)\leq \frac{\sup_{x\in\reals^d}\maxEigenvalue{\gradient{}^2f(x)}}{2}\norm{x}^2.
\end{equation*}
Then, 
\begin{equation*}
\begin{aligned}[b]
    \kappa
    &= \limsup_{\norm{x}\to \infty}\frac{f(x)}{\norm{x}^2}
    \\
    &\leq \limsup_{\norm{x}\to \infty}\frac{f(0)+\innerProduct{\gradient{}f(0)}{x}+\frac{1}{2}\sup_{x\in\reals^d}\maxEigenvalue{\gradient{}^2 f(x)}\norm{x}^2}{\norm{x}^2}
    \\
    &=\frac{1}{2}\sup_{x\in\reals^d}\maxEigenvalue{\gradient{}^2 f(x)}.
\end{aligned}
\end{equation*}
\end{proof}

By \cite[Corollary 1]{Gao2016}, the existence of an optimal $\mu^\ast$ implies that $\lambda^\ast\geq\kappa$. Under the additional assumption that $\lambda^\ast\neq\kappa$, we can show that optimal solutions of \eqref{eq:dro reformulation} satisfy necessary conditions for optimality:

\begin{proposition}\label{prop:relation classical dro}
Let $\refmu\in\Ppabs{2}{\reals^d}$ be absolutely continuous, assume the supremum in \eqref{eq:dro reformulation} is finite and attained, and 
\begin{equation*}
    \kappa=\sup_{x\in\reals^d}\frac{\maxEigenvalue{{\gradient{}^2f(x)}}}{2}.
\end{equation*}
Let $\lambda^\ast>\kappa$ be a strictly positive optimal solution and consider the well-defined diffeomorphism
\begin{equation*}
    T(x)=\left(\Id-\frac{1}{2\lambda^\ast}\gradient{}f\right)^{-1}(x).
\end{equation*}
Then, $\mu^\ast\coloneqq\pushforward{T}\refmu\in\Pp{2}{\reals^d}$ attains the supremum in \eqref{eq:dro reformulation} and solves the optimality conditions of \cref{thm:wasserstein lagrange multipliers} with $\lambda=\lambda^\ast$.
\end{proposition}

The proof relies on the following technical lemma: 

\begin{lemma}\label{lemma:diffeo}
Let $\varphi\in\Ctwo{\reals^d}$ be strongly convex and $T\coloneqq\gradient{}\varphi$. Then, $T$ is $\Cone{}$-diffeormorphism. Moreover, $T^{-1}$ is the gradient of a strongly convex function.
\end{lemma}

\begin{proof}\
\begin{enumerate}
    \item $T$ is a diffeomorphism:
    By the Hadamard-Caccioppoli theorem~\cite{Gordon1972}, we can show that $T$ is (topologically) proper and that its Jacobian is invertible for all $x\in\reals^d$. Invertibility of the Jacobian of $T$ follows directly from $\varphi$ being strongly convex: since $\gradient{}^2T(x)-\alpha\eye{}$ is positive semidefinite for some $\alpha>0$, all eigenvalues of $\gradient{}^2T(x)$ are larger than $\alpha$, and thus never zero (which implies invertibility). 
    Thus, it suffices to prove that $T$ is proper; i.e., that the preimage of compact set is compact or, equivalently, that $\norm{T(x)}\to+\infty$ as $\norm{x}\to+\infty$. It is well-known that gradients of strongly convex functions are strongly monotone, such that
    \begin{equation*}
        \innerProduct{T(x)-T(0)}{x-0}\geq\alpha\norm{x-0}^2
    \end{equation*}
    for some $\alpha>0$. 
    By Cauchy-Schwartz, $\innerProduct{T(x)-T(0)}{x-0}\leq \norm{T(x)-T(0)}\norm{x}$ and thus
    \begin{equation*}
        \norm{T(x)-T(0)}\geq\alpha\norm{x}.
    \end{equation*}
    Finally, by triangle inequality, $\norm{T(x)}\geq\norm{T(x)-T(0)}-\norm{T(0)}$, which implies
    \begin{equation*}
        \norm{T(x)}\geq\alpha\norm{x}-\norm{T(0)}.
    \end{equation*}
    Clearly, $\norm{T(x)}\to\infty$ as $\norm{x}\to\infty$, which concludes the proof. 

    \item $T^{-1}$ is the gradient of a strongly convex function: it suffices to prove $\gradient{}T^{-1}$ symmetric and that $\gradient{}T^{-1}-\beta\eye{}$ is positive semidefinite for some $\beta>0$. By the inverse function theorem
    \begin{equation*}
        \gradient{}T^{-1}(x)=\left(\gradient{}T(T^{-1}(x))\right)^{-1},
    \end{equation*}
    which is symmetric since $\gradient{}T=\gradient{}^2\varphi$ is symmetric and the inverse of symmetric matrices is symmetric. Moreover, for all $x\in\reals^d$
    \begin{equation*}
        \minEigenvalue{\gradient{}T^{-1}(x)}
        =
        \frac{1}{\maxEigenvalue{\gradient{}T(T^{-1}(x))}}\geq\frac{1}{\alpha}>0.
    \end{equation*}
    Thus, $\gradient{}T^{-1}-\frac{1}{\alpha}\eye{}$ is positive semidefinite, and, since $\frac{1}{\alpha}>0$, we conclude.
\end{enumerate}
\end{proof}

\begin{proof}[Proof of \cref{prop:relation classical dro}]
We proceed in five steps: 
\begin{enumerate}
    \item 
    $T$ is a well-defined $\Cone{}$-diffeomorphism: As the inverse of a diffeomorphism is a diffeomorphism, it suffices to prove that $\Id-\frac{1}{2\lambda^\ast}\gradient{}f$ is a $\Cone{}$-diffeomorphism. By \cref{lemma:diffeo}, it is enough to show that $\Id-\frac{1}{2\lambda^\ast}\gradient{}f$ is the gradient of a strongly convex function or equivalently that all eigenvalues of its Jacobian are larger by some $\alpha>0$ for all $x\in\reals^d$. Note that  
    \begin{equation*}
        \gradient{}\left(\Id-\frac{1}{2\lambda^\ast}\gradient{}f\right)(x)
        =
        \eye{}-\frac{1}{2\lambda^\ast}\gradient{}^2f(x).
    \end{equation*}
    Clearly,
    \begin{equation*}
        \spec\left(\eye{}-\frac{1}{2\lambda^\ast}\gradient{}^2f(x)\right)
        =
        1-\frac{1}{2\lambda^\ast}\spec(\gradient{}^2f(x)).
    \end{equation*}
    Since $\maxEigenvalue{\gradient{}^2f(x)}\leq2\kappa$ uniformly and $\gradient{}^2f(x)$ is symmetric for all $x\in\reals^d$, we have
    \begin{equation*}
        \frac{1}{2\lambda^\ast}\spec(\gradient{}^2f(x))
        \subseteq\frac{1}{2\lambda^\ast}(-\infty,2\kappa]
        =\left(-\infty,\frac{\kappa}{\lambda^\ast}\right]
        \subsetneq(-\infty,1)
        \quad\forall x\in\reals^d,
    \end{equation*}
    and so $\minEigenvalue{\eye{}-\frac{1}{2\lambda^\ast}\gradient{}^2f(x)}\geq 1-\kappa/\lambda^\ast>0$ uniformly. So, $\alpha=1-\kappa/\lambda^\ast>0$.
    
    \item
    $T$ is the optimal transport map from $\refmu$ to $\mu^\ast$: By \cref{lemma:diffeo}, $T^{-1}$ is the gradient of a (strongly) convex function, thus, by \cref{prop:brenier2}, it is the optimal transport map from $\refmu$ and $\mu^\ast$. 
    
    \item 
    $\mu^\ast$ satisfies the optimality conditions with $\lambda^\ast$: recall the the gradient of the objective function is $\gradient{}f$ and that the gradient of the Wasserstein distance is $2(\Id-\optMap{\mu^\ast}{\refmu})=2(\Id-T^{-1})$. It is readily verified that 
    \begin{equation*}
        \gradient{}f=2\lambda\left(\Id - T^{-1}\right).
    \end{equation*}

    \item
    $\mu^\ast$ lies on the boundary of the Wasserstein ball: we need to show that $\wassersteinDistance{2}{\mu^\ast}{\refmu}=\varepsilon$. To start, note that the function $x'\mapsto\lambda\norm{x-x'}^2-f(x')$ is strongly convex in $x$ (for all $x$ and $\lambda$) and thus the function $\lambda\mapsto \min_{x'\in\reals^d}\lambda\norm{x-x'}^2-f(x)$ is continuously differentiable around $\lambda^\ast$ for all $x\in\reals^d$; see~\cite[Theorems 4.13 and 4.14]{Bonnans2000}. So, by Leibniz integration rule, the function
    \begin{equation*}
        \lambda\mapsto \int_{x\in\reals^d}\min_{x'\in\reals^d}\lambda\norm{x-x'}^2-f(x)\d\mu(x)
    \end{equation*}
    is differentiable around $\lambda^\ast$. Indeed, $(\Id-\frac{1}{2\lambda}\gradient{}f)^{-1}$ remains a well defined diffeomorphism for $\lambda$ sufficiently close to $\lambda^\ast$. In particular, it is, by continuity, pointwise dominated by an integrable function and its derivative exists. 
    So, a necessary condition for optimality of the dual reads
    \begin{equation*}
    \begin{aligned}
        \varepsilon^2
        &=
        \diff{}{\lambda}\int_{\reals^d}\lambda\norm{x-\left(\Id-\frac{1}{2\lambda} \gradient{} f\right)^{-1}(x)}^2-f\left(\left(\Id-\frac{1}{2\lambda} \gradient{} f\right)^{-1}(x)\right)\d\refmu(x)
        \\
    \end{aligned}
    \end{equation*}
    Reuse Leibniz integration rule to exchange derivative and integration we obtain
    \begin{equation*}
    \begin{aligned}
        \varepsilon^2
        &=
        \int_{\reals^d}\diff{}{\lambda}\lambda\norm{x-\left(\Id-\frac{1}{2\lambda} \gradient{} f\right)^{-1}(x)}^2-f\left(\left(\Id-\frac{1}{2\lambda} \gradient{} f\right)^{-1}(x)\right)\d\refmu(x)
        \\
        &=
        \begin{aligned}[t]
        &\int_{\reals^d}\norm{x-\left(\Id-\frac{1}{2\lambda}\gradient{} f\right)^{-1}(x)}^2\d\refmu(x)
        \\
        &+2\lambda\int_{\reals^d}
        \left(\left(\Id-\frac{1}{2\lambda} \gradient{} f\right)^{-1}(x)-x\right)\left(\diff{}{\lambda}\left(\Id-\frac{1}{2\lambda} \gradient{} f\right)^{-1}(x)\right)\d\refmu(x)
        \\
        &-2\lambda\int_{\reals^d}\frac{1}{2\lambda}\gradient{}f\left(\left(\Id-\frac{1}{2\lambda} \gradient{} f\right)^{-1}(x)\right)\left(\diff{}{\lambda}\left(\Id-\frac{1}{2\lambda} \gradient{} f\right)^{-1}(x)\right)\d\refmu(x)
        \end{aligned}
        \\
        &=
        \int_{\reals^d}\norm{x-\left(\Id-\frac{1}{2\lambda}\gradient{} f\right)^{-1}(x)}^2\d\refmu(x)
        \\
        &=
        \wassersteinDistance{2}{\mu^\ast}{\refmu}^2,
    \end{aligned}
    \end{equation*}    
    where we used $(\Id-\frac{1}{2\lambda}\gradient{}f)((\Id-\frac{1}{2\lambda}\gradient{} f)^{-1}(x))=x$. Note that this directly implies that $\mu^\ast\in\Pp{2}{\reals}$ by triangle inequality. 

    \item 
    $\mu^\ast$ is optimal: it suffices to check that the cost resulting from $\mu^\ast$ coincides the with optimal value of the dual problem. First, basic rules of integration give
    \begin{equation*}
    \begin{aligned}
        \expectedValue{\mu^\ast}{f(x)}
        &=
        \int_{\reals^d}f(x)\d\left(\pushforward{T}\refmu\right)(x)
        \\
        &=
        \int_{\reals^d}f(T(x))\d\refmu(x).
        \\
        &=
        \lambda^\ast\int_{x\in\reals^d}\norm{x-T(x)}^2\d\refmu(x)
        +
        \int_{x\in\reals^d}
        -\lambda^\ast\norm{x-T(x)}^2+f(T(x))\d\refmu(x).
    \end{aligned}
    \end{equation*}
    By definition of $T$ for fixed $x\in\reals^d$, we have
    \begin{equation*}
        \max_{x'\in\reals^d}-\lambda^\ast\norm{x-x'}^2+f(x')
        =
        -\lambda^\ast\norm{x-T(x)}^2+f\left(T(x)\right),
    \end{equation*}
    where we used that the maximum is attained at $x'=T(x)$.
    Thus, 
    \begin{equation*}
    \begin{aligned}[b]
        \expectedValue{\mu^\ast}{f(x)}
        &=
        \lambda^\ast\int_{x'\in\reals^d}\norm{x-T(x)}^2\d\refmu(x)
        +
        \int_{x\in\reals^d}
        \max_{x\in\reals^d}-\lambda^\ast\norm{x-x'}^2+f(x')\d\refmu(x)
        \\
        &=
        \lambda^\ast\wassersteinDistance{2}{\mu^\ast}{\refmu}^2-\int_{\reals^d}\min_{x'\in\reals^d}\lambda^\ast\norm{x-x'}^2-f(x')\d\refmu(x)
        \\
        &=
        \lambda^\ast\varepsilon^2-\int_{\reals^d}\min_{x'\in\reals^d}\lambda^\ast\norm{x-x'}^2-f(x')\d\refmu(x).
    \end{aligned}
    \end{equation*}
\end{enumerate}
\end{proof}

The proof directly reveals the following corollary:

\begin{corollary}\label{cor:relation classical dro}
Let the assumptions of \cref{prop:relation classical dro} hold. Then, there exists a $\mu^\ast$ attaining the supremum which is absolutely continuous. 
\end{corollary}

\begin{proof}
Since $T$ is a diffeomorphism (in particular, it is injective and the Jacobian has non-zero determinant) and $\refmu$ is absolutely continuous, $\mu^\ast$ is absolutely continuous~\cite[Lemma 5.5.3]{Ambrosio2008a}.
\end{proof}

\begin{remark}\
\begin{enumerate}
    \item
    Many relevant functions satisfy the assumption $\kappa\geq\sup_{x\in\reals^d}\frac{\maxEigenvalue{\gradient{}^2f}}{2}$:
    \begin{enumerate}
        \item linear functions: $\kappa=0$ and $\gradient{}^2f(x)$ is the zero matrix;
        
        \item convex functions whose growth at infinity upper bounds their Hessian (e.g., quadratic functions, but not convex functions such as $x^2+e^{-x^2}$);
        
        \item concave functions: see \cref{prop:relation classical dro concave} for details;
        
        \item functions with norm of the Hessian uniformly bounded via $\frac{1}{2}\sup_{x\in\reals^d}\norm{\gradient{}^2f}\leq\kappa$. 
    \end{enumerate}
    
    \item 
    By \cite[Corollary 1]{Gao2016} an optimal solutions exists only if $\lambda^\ast=0$ or $\lambda^\ast\geq\kappa$. Instead, \cref{prop:relation classical dro} assumes $\lambda^\ast>\kappa$. The case $\lambda^\ast=0$ can be ruled out assuming that the maximum of the unconstrained problem does not lie in the Wasserstein ball; the case $\lambda^\ast=\kappa$ is degenerate and needs to be examined individually.   
    
    \item
    One can replace the assumption $\kappa=\sup_{x\in\reals^d}\frac{\maxEigenvalue{\gradient{}^2f}}{2}$ with the assumption that there exists optimal $\lambda^\ast$ such that $\lambda^\ast>\sup_{x\in\reals^d}\frac{\maxEigenvalue{\gradient{}^2f}}{2}$. Yet, there might not exist a $\lambda^\ast>0$ satisfying the equation.
\end{enumerate}
\end{remark}

The proof can be further strengthened (including $\lambda^\ast=\kappa$) if we additionally assume that $f$ is concave in $x$: 

\begin{proposition}\label{prop:relation classical dro concave}
Let $f\in\Ctwo{\reals}$ and $\refmu\in\Ppabs{2}{\reals^d}$. Assume $f$ is concave. Let $\lambda^\ast\geq\kappa$ be a strictly positive optimal solution and consider the well-defined diffeomorphism
\begin{equation*}
    T(x)=\left(\Id-\frac{1}{2\lambda^\ast}\gradient{}f\right)^{-1}(x).
\end{equation*}
Then, $\mu^\ast\coloneqq\pushforward{T}\refmu\in\Pp{2}{\reals^d}$ attains the supremum in \eqref{eq:dro reformulation} and solves the optimality conditions of \cref{thm:wasserstein lagrange multipliers} with $\lambda=\lambda^\ast$.
\end{proposition}

\begin{proof}
It suffices to show that $\Id-\frac{1}{2\lambda^\ast}\gradient{}f$ is the gradient of a strongly convex function. Then, the proof is identical to the proof of \cref{prop:relation classical dro}. For this, simply observe that, by concavity, all eigenvalue of $\gradient{}^2f(x)$ are non-negative, and thus
\begin{equation*}
    \spec\left(I-\frac{1}{2\lambda^\ast}\gradient{}^2f(x)\right)
    =
    1-\frac{1}{2\lambda^\ast}\spec(\gradient{}^2f(x))
\end{equation*}
and thus $\minEigenvalue{\eye{}-\frac{1}{2\lambda^\ast}\gradient{}f(x)}\geq 1$ for all $x\in\reals^d$. Thus, $\Id-\frac{1}{2\lambda^\ast}\gradient{}f$ is strongly convex.
\end{proof}

Again, proof directly reveals the following corollary, whose proof is identical to the proof \cref{cor:relation classical dro}:

\begin{corollary}\label{cor:relation classical dro concave}
Let the assumptions of \cref{prop:relation classical dro concave} hold. Then, there exists a $\mu^\ast$ attaining the supremum which is absolutely continuous. 
\end{corollary}

\begin{remark}
This result mirrors point (iii) in \cite[Theorem 1]{Gao2016}, stating that, when $f$ is convex, one can restrict the attention to optimal transport maps.
\end{remark}

\begin{comment}
\subsection{Moment-based Ambiguity Sets}
\nlmargin{Consider}{needs to be improved and made meaningful} now the moment-constrained optimization problem
\begin{equation}\label{eq:dro moments}
    \min_{w\in\mathcal{W}}\sup_{\mu\in\mathcal{D}}\expectedValue{\mu}{\innerProduct{w}{x}}+\weight\variance{\mu}{\innerProduct{w}{x}}
\end{equation}
where is
\begin{equation*}
    \mathcal{D}
    \coloneqq 
    \left\{\mu\in\Pp{2}{\reals^d}:\expectedValue{\mu}{\frac{1}{2}\norm{Ax-b}^2}=0\right\}.
\end{equation*}
\end{comment}



\subsection{Solving the \gls{acr:dro} Problem}
So far, we reviewed methods to solve the inner optimization problem~\eqref{eq:general dro}. In this section, we show how this result can be deployed to solve \eqref{eq:general dro} and compute the optimal $w^\ast$. We make the following standard assumption:
\begin{assumption}\label{assumption:regularity full dro}
$\cost(\cdot,\mu)$ is convex and continuously differentiable for all $\mu$ and $w\mapsto\gradient{w}\cost(w,\mu)$ is Lipschitz continuous and bounded by $L$ (uniformly in $\mu$). Finally, $\mathcal{W}$ is convex compact.
\end{assumption}
\cref{assumption:regularity full dro} immediately implies existence of a solution of \cref{eq:general dro}.
For simplicity, let us define
\begin{equation}
\begin{aligned}
    \phi(w)&\coloneqq\max_{\mu\in\closedWassersteinBall{2}{\radius}{\refmu}}\cost(w,\mu) \\
    \mu^\ast(w)&\in\arg\max_{\mu\in\closedWassersteinBall{2}{\radius}{\refmu}}\cost(w,\mu).
\end{aligned}
\end{equation} 
Evaluations of $\phi$ are easy and rely on the theory presented before. 
The next lemma is immediate. 
\begin{lemma}
The function $w\mapsto\phi(w)$ is convex.
\end{lemma}
\begin{proof}
The lemma follows directly from the well-known fact that the supremum of convex functions is convex. 
\end{proof}
While convex, $\phi(w)$ is generally non-differentiable, regardless of the smoothness of $\cost$. Fortunately, we can still prove convergence:
\newcommand{\wopt}{w^\ast}
\newcommand{\wset}{\mathcal{W}}
\newcommand{\witer}[1]{w_{#1}}
\newcommand{\muiter}[1]{\mu^\ast(\witer{#1})}
\newcommand{\stepsizeiter}[1]{\eta_{#1}}
\begin{theorem}[Convergence]
Let $(\stepsizeiter{k})_{k\in\naturals}$ be a sequence of strictly positive real step sizes. Assume
\begin{equation*}
\stepsizeiter{k}\to 0 \text{ and }\sum_{k=0}^\infty\stepsizeiter{k}=\infty.
\end{equation*}
Consider the sequence $(\witer{k})_{k\in\mathbb{N}}$ generated by
\begin{equation}\label{eq:algorithm}
    \witer{k+1}=\projection{\wset}{\witer{k}-\stepsizeiter{k}\gradient{w}\cost(\witer{k},\muiter{k})}
\end{equation}
with $\witer{0}\in\wset$. Then,
\begin{equation*}
    \min_{i=0,\ldots,k}\phi(\witer{i})\to\phi(\wopt) \text{ as } k\to\infty.
\end{equation*}
\end{theorem}
\begin{proof}
The proof follows along the lines of proofs of convergence of subgradient methods.
\begin{comment}
\begin{equation*}
\begin{aligned}
    \phi(\witer{k+1})
    &=
    \max_{\mu\in\closedWassersteinBall{2}{\radius}{\refmu}}J(\witer{k+1},\mu)
    \\
    &\geq
    \cost(\witer{k+1},\muiter{k}) 
    \\
    &\geq 
    \cost(\witer{k},\muiter{k}) + \innerProduct{\gradient{w}J(\witer{k},\muiter{k})}{\witer{k+1}-\witer{k}}
    \\
    &
    =
    \phi(\witer{k}) - \stepsizeiter{k}\norm{\gradient{w}\cost(\witer{k},\muiter{k}}^2,
\end{aligned} 
\end{equation*}
\end{comment}
To start, we use convexity and differentiability of $\cost(\cdot,\mu)$:
\begin{equation}\label{eq:proof algorithm 1}
\begin{aligned}
    \phi(\wopt)
    &=
    \max_{\mu\in\closedWassersteinBall{2}{\radius}{\refmu}}J(\wopt,\mu)
    \\
    &\geq
    \cost(\wopt,\muiter{k}) 
    \\
    &\geq 
    \cost(\witer{k},\muiter{k}) + \innerProduct{\gradient{w}J(\witer{k},\muiter{k})}{\wopt-\witer{k}}
    \\
    &= 
    \phi(\witer{k}) + \innerProduct{\gradient{w}J(\witer{k},\muiter{k})}{\wopt-\witer{k}}.
\end{aligned} 
\end{equation}
Moreover, by non-expansiveness of the projection operator, we get
\begin{equation*}
\begin{aligned}
    \norm{\witer{k+1}-\wopt}^2
    &=
    \norm{\projection{\wset}{\witer{k}-\stepsizeiter{k}\gradient{w}\cost(\witer{k},\muiter{k})}-\projection{\wset}{\wopt}}^2
    \\
    &\leq 
    \norm{\witer{k}-\stepsizeiter{k}\gradient{w}\cost(\witer{k},\muiter{k})-\wopt}^2
    \\
    &=
    \norm{\witer{k}-w^\ast}^2 - 2\stepsizeiter{k}\innerProduct{\gradient{w}\cost(\witer{k},\muiter{k})}{\witer{k}-\wopt}+\stepsizeiter{k}^2\norm{\gradient{w}\cost(\witer{k},\muiter{k})}^2
    \\
    &\leq 
    \norm{\witer{k}-w^\ast}^2 + 2\stepsizeiter{k}(\phi(\wopt)-\phi(\witer{k}))+\stepsizeiter{k}^2\norm{\gradient{w}\cost(\witer{k},\muiter{k})}^2,
\end{aligned}
\end{equation*}
where the last inequality follows from \eqref{eq:proof algorithm 1}.
An inductive argument then leads to 
\begin{equation*}
\begin{aligned}
    \norm{\witer{k+1}-\wopt}^2
    &\leq
    \norm{\witer{1}-\wopt}^2+2\sum_{i=0}^{k}\stepsizeiter{i}\left(\phi(\wopt)-\phi(\witer{i})\right)+\sum_{i=0}^k\stepsizeiter{i}^2\norm{\gradient{w}\cost(\witer{i},\muiter{i})}^2,
\end{aligned}
\end{equation*}
and so to
\begin{equation*}
\begin{aligned}
    2\sum_{i=1}^{k}\stepsizeiter{i}\left(\phi(\witer{i})-\phi(\wopt)\right)
    &\leq
    \norm{\witer{1}-\wopt}^2-\norm{\witer{k+1}-\wopt}^2+\sum_{i=0}^{k}\stepsizeiter{i}^2\norm{\gradient{w}\cost(\witer{i},\muiter{i})}^2
    \\
    &\leq
    \norm{\witer{1}-\wopt}^2+L^2\sum_{i=1}^{k}\stepsizeiter{i}^2.
\end{aligned}
\end{equation*}
As trivially $\min_{i=0,\ldots,k}\phi(\witer{i})-\phi(\wopt)\leq \phi(\witer{i})-\phi(\wopt)$ for all $i$ we therefore conclude
\begin{equation*}
\begin{aligned}
    \min_{i=0,\ldots,k}\phi(\witer{i})-\phi(\wopt)
    \leq 
    \frac{\norm{\witer{1}-\wopt}^2+L^2\sum_{i=0}^{k}\stepsizeiter{i}^2}{2\sum_{i=0}^k\stepsizeiter{i}}.
\end{aligned}
\end{equation*}
The result follows via the assumptions on the step size.
\end{proof}

\begin{remark}\
\begin{enumerate}
    \item In the cases of the mean and mean-variance functionals, it is easy to find (uniform) upper bounds for the gradient.
    
    \item Iteration \eqref{eq:algorithm} resembles a saddle flow with infinitely fast gain for the probability distribution $\mu_k$ (cf. dual ascent methods).
\end{enumerate}
\end{remark}
